# Supplementary material for: SNAP: Towards Segmenting Anything in Any Point Cloud
Source: arXiv:2510.11565 source file (2026-02-10)

Ground-Truth Mask

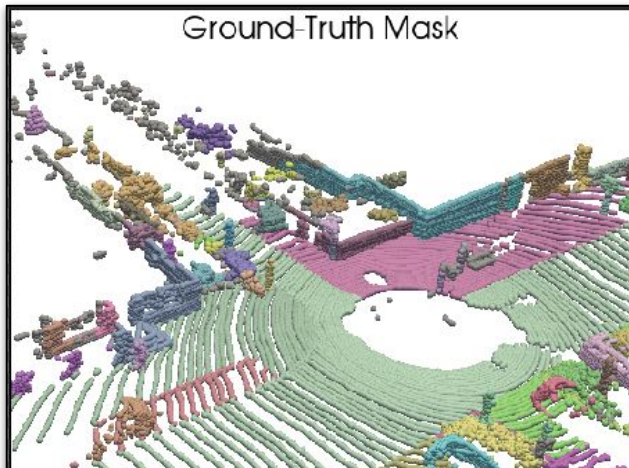

1-Click Mask, Mean IoU: 0.69

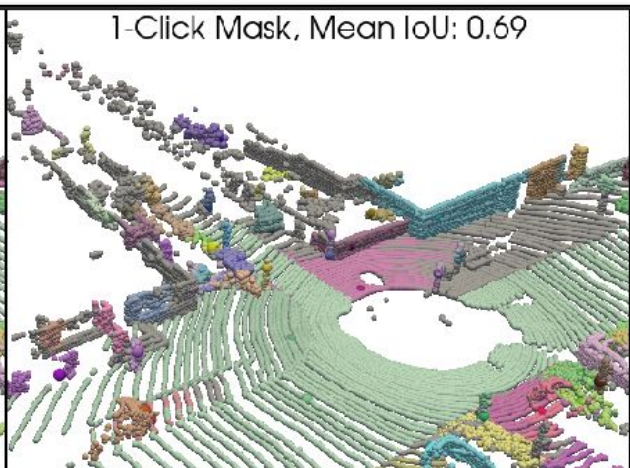

5-Click Mask, Mean IoU: 0.87

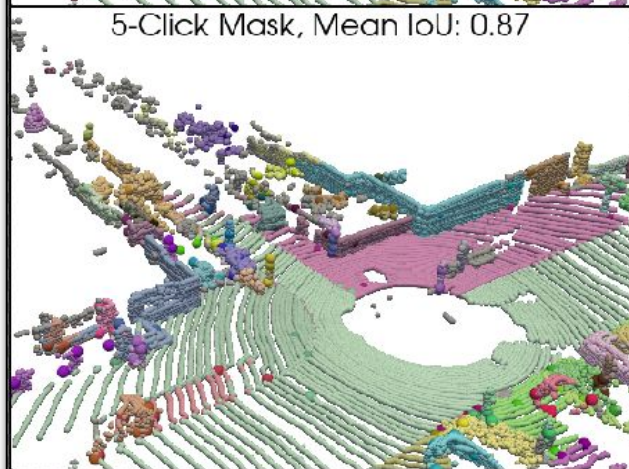

10-Click Mask, Mean IoU: 0.90

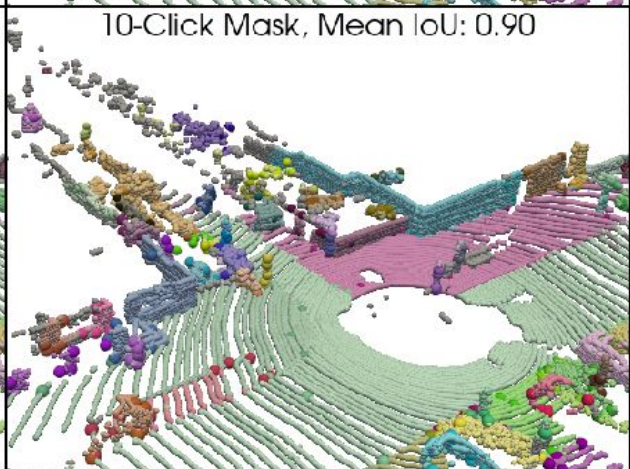

Ground-Truth Mask

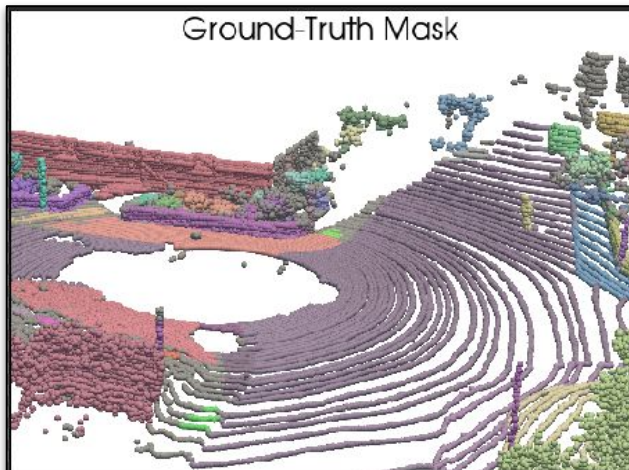

1-Click Mask, Mean IoU: 0.60

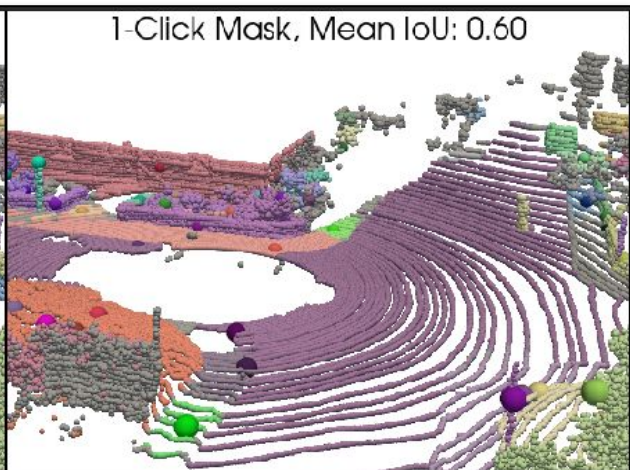

5-Click Mask, Mean IoU: 0.83

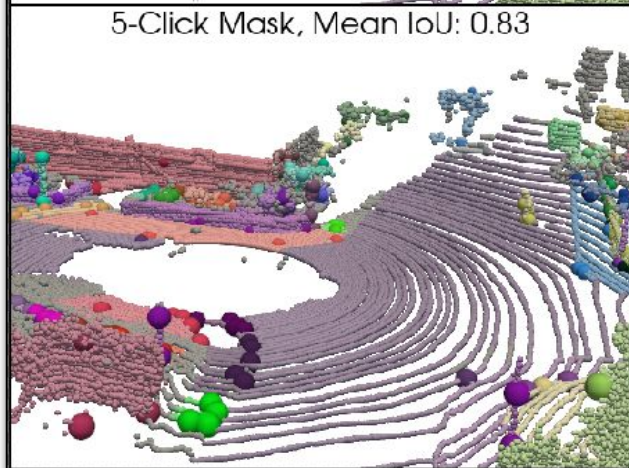

10-Click Mask, Mean IoU: 0.87

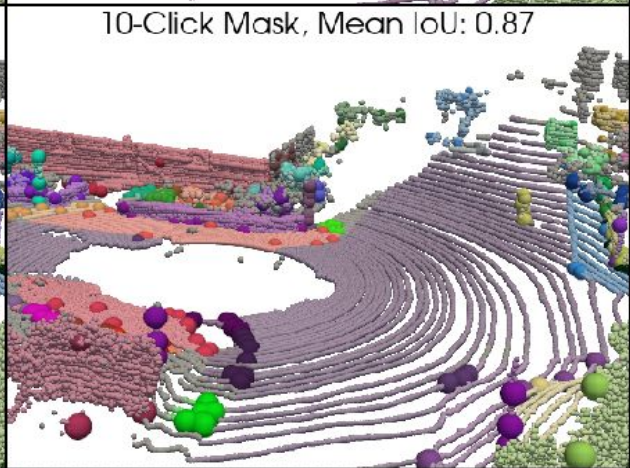



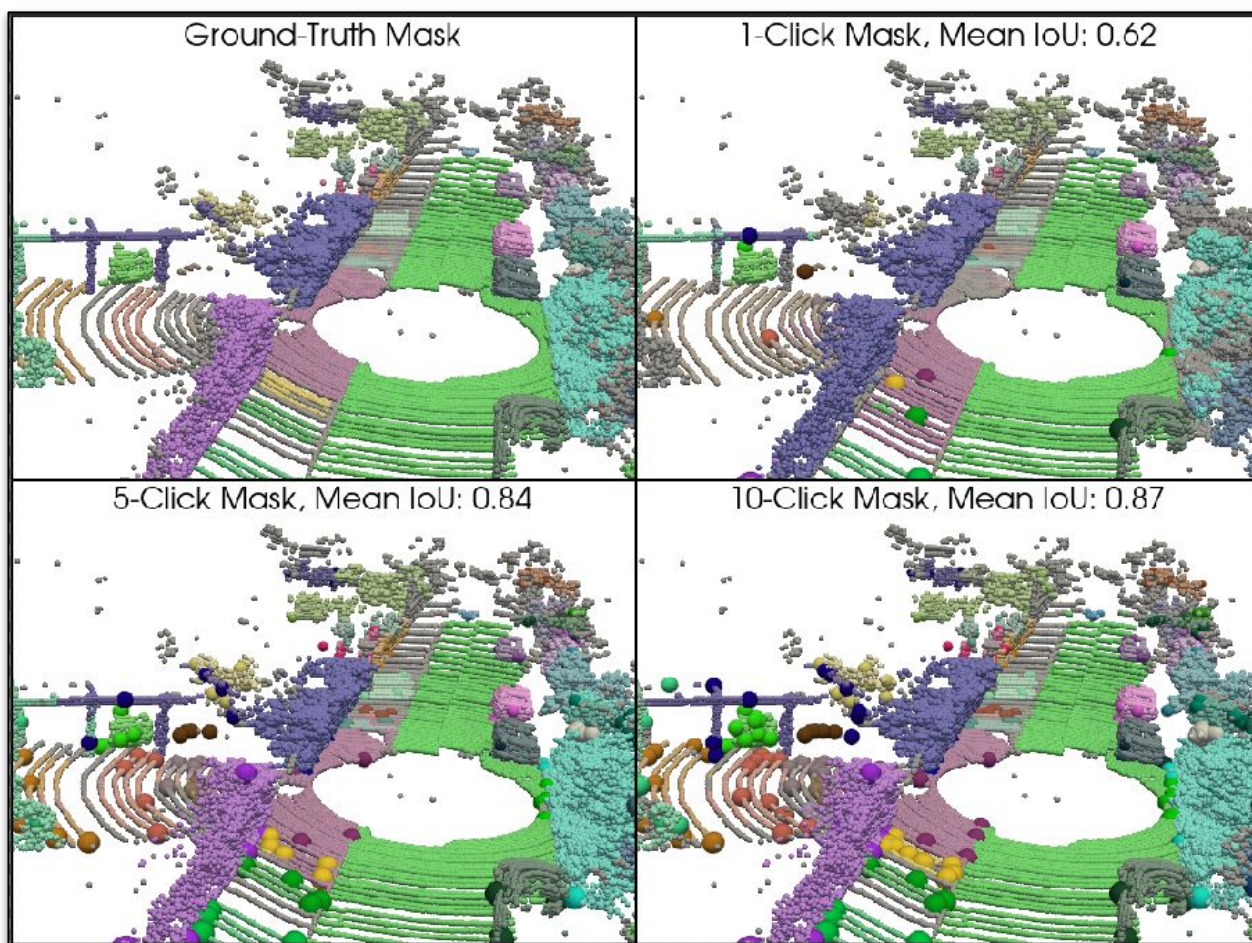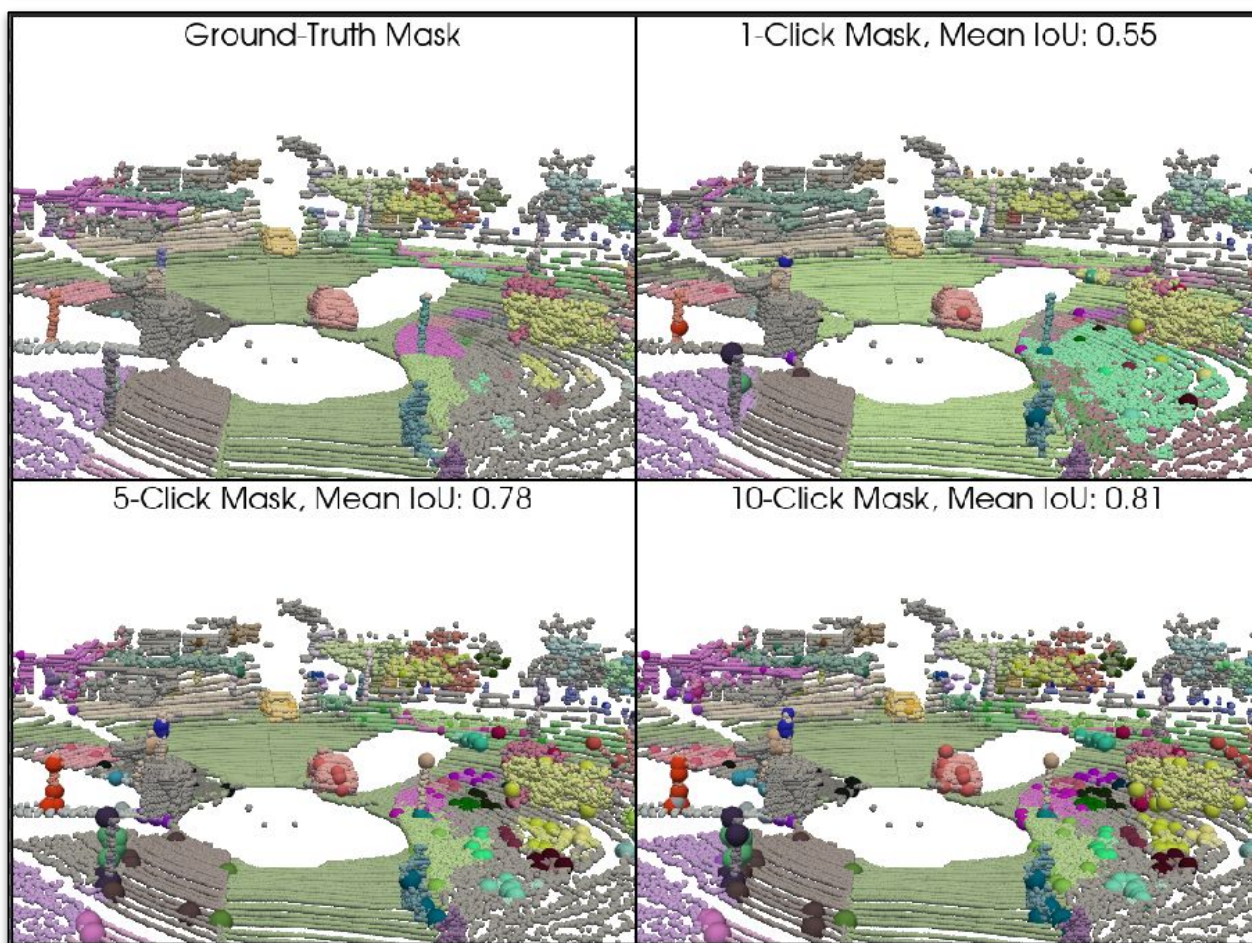



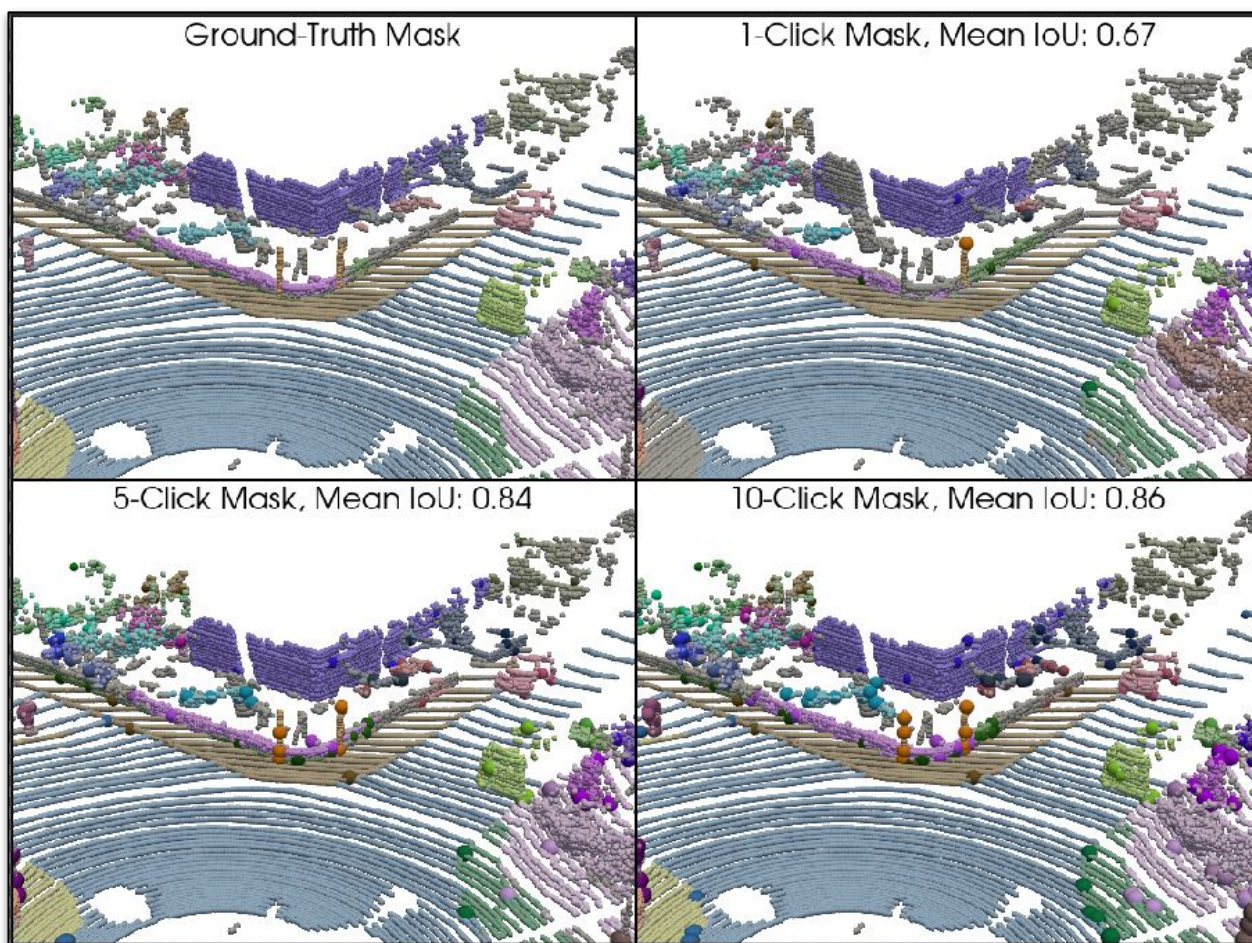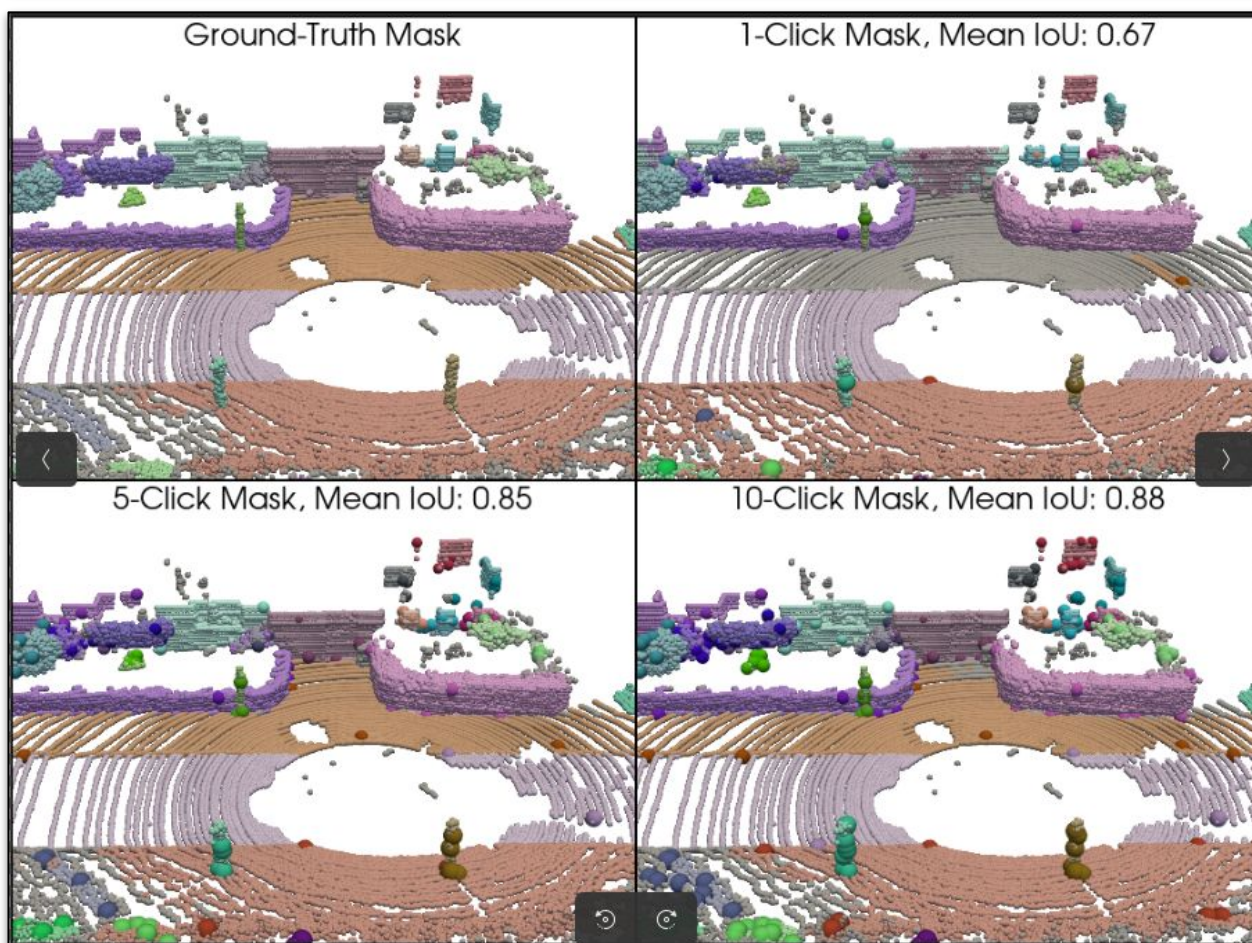

Supplement: Supplementary file 1 [file supp_outdoor-3.pdf]
